# Supplementary material for: Robust Reinforcement Learning Objectives for Sequential Recommender Systems
Source: arXiv:2305.18820 source file (2024-04-18)
Supplement: Supplementary file 1 [file appendices.tex]

\newpage
\appendix
